# Supplementary material for: Certified Distributional Robustness on Smoothed Classifiers
Source: arXiv:2010.10987 source file (2021-04-30)
Supplement: Supplementary file 1 [file supplemental.tex]

\typeout{IJCAI--21 Instructions for Authors}

% These are the instructions for authors for IJCAI-21.

\documentclass{article}
\pdfpagewidth=8.5in
\pdfpageheight=11in
% The file ijcai21.sty is NOT the same than previous years'
\usepackage{ijcai21}

% Use the postscript times font!
\input{math_commands.tex}
\usepackage{times}
\usepackage{soul}
\usepackage{url}
\usepackage[hidelinks]{hyperref}
\usepackage[utf8]{inputenc}
\usepackage[small]{caption}
\usepackage{graphicx}
\usepackage{amsmath}
\usepackage{amsthm}
\usepackage{booktabs}
\usepackage{algorithm}
\usepackage{algorithmic}
\urlstyle{same}

% Optional math commands from https://github.com/goodfeli/dlbook_notation.
\usepackage[T1]{fontenc}
\usepackage{bm}
\usepackage{subfigure}
\usepackage{wrapfig}
\usepackage{helvet} % DO NOT CHANGE THIS
\usepackage{courier}  % DO NOT CHANGE THIS
\usepackage{graphicx} % DO NOT CHANGE THIS
\usepackage{caption} % DO NOT CHANGE THIS AND DO NOT ADD ANY OPTIONS TO IT
\frenchspacing  % DO NOT CHANGE THIS
\usepackage{amssymb}
\usepackage{latexsym}
\usepackage{bbding}
\usepackage{booktabs}%表格竖线
\usepackage{multirow}
\usepackage{color}
\usepackage{authblk}
%\usepackage[utf8]{inputenc}

%\newtheorem{proof}{\bf Proof}
%\DeclareMathOperator*{\argmax}{argmax}

%PDF Info Is REQUIRED.
%\pdfinfo{
%	/TemplateVersion (IJCAI.2021.0)
%}
\begin{document}

\title{Supplementary Materials}
\author{}
% make the title area
\maketitle

\appendix
\input{appendix}
\input{appendix_B}
\bibliographystyle{named}
\bibliography{main}

\end{document}
